# Supplementary material for: A Realization of the Haldane-Kane-Mele Model in a System of Localized Spins
Source: arXiv:1603.04827 source file (2016-09-20)
Supplement: Supplementary file 1 [file SOM.pdf]

# A Realization of the Haldane-Kane-Mele Model in a System of Localized Spins

## Supplementary Material

Se Kwon Kim, Héctor Ochoa, Ricardo Zarzuela, and Yaroslav Tserkovnyak
*Department of Physics and Astronomy, University of California, Los Angeles, California 90095, USA*

### Experimental realization of the model: Basic formalism

The proposed minimal Hamiltonian can be recast as

$$H = H_e + J\,\mathbf{S}_i \cdot \mathbf{s}\left(\mathbf{R}_i\right), \tag{1}$$

where the first term describes the dynamics of the itinerant electrons that mediate the interaction, and the second term is just the exchange coupling between the localized spins and the spin density of the Fermi sea. The latter is defined as

$$\mathbf{s}\left(\mathbf{R}_i\right) = \sum_{\mathbf{r}} \delta^{(2)}\left(\mathbf{r} - \mathbf{R}_i\right) \boldsymbol{\sigma}\left(\mathbf{r}\right), \tag{2}$$

where $\boldsymbol{\sigma}$ is the vector of Pauli matrices. To the lowest order in the exchange constant $J$, the RKKY Hamiltonian for the localized spins reads

$$H_{\text{RKKY}} = J^2 \sum_{i,j} \chi_{\alpha,\beta}\left(\mathbf{R}_i, \mathbf{R}_j\right) S_i^\alpha S_j^\beta, \tag{3}$$

where the zero frequency spin susceptibility can be computed as

$$\chi_{\alpha,\beta}\left(\mathbf{R}_i, \mathbf{R}_j\right) \equiv -\frac{1}{2\pi} \int_{-\infty}^{\epsilon_F} d\omega \,\text{Im Tr}\left[\sigma_\alpha \hat{G}^R\left(\mathbf{R}_i, \mathbf{R}_j, \omega\right) \sigma_\beta \hat{G}^R\left(\mathbf{R}_j, \mathbf{R}_i, \omega\right)\right]. \tag{4}$$

The retarded Green operator in spin space is defined as

$$\hat{G}^R\left(\mathbf{R}_i, \mathbf{R}_j, \omega\right) \equiv \langle \mathbf{R}_i | \left(\omega + i0^+ - \mathcal{H}_e\right)^{-1} | \mathbf{R}_j \rangle. \tag{5}$$

Since the (mirror) symmetry $z \to -z$ should be preserved in the spin model, the $z$-component of electron spin is a good quantum number. Therefore, the retarded Green function admits the decomposition

$$\hat{G}^R\left(\mathbf{R}_i, \mathbf{R}_j, \omega\right) = \left[G_\uparrow^R\left(\mathbf{R}_i, \mathbf{R}_j, \omega\right) + G_\downarrow^R\left(\mathbf{R}_i, \mathbf{R}_j, \omega\right)\right] \sigma_0 + \left[G_\uparrow^R\left(\mathbf{R}_i, \mathbf{R}_j, \omega\right) - G_\downarrow^R\left(\mathbf{R}_i, \mathbf{R}_j, \omega\right)\right] \sigma_z. \tag{6}$$

The RKKY Hamiltonian becomes then

$$H_{\text{RKKY}} = \sum_{i,j} J_{ij}^H \mathbf{S}_i \cdot \mathbf{S}_j + J_{ij}^I S_i^z S_j^z + J_{ij}^{DM} \hat{\mathbf{z}} \cdot \left(\mathbf{S}_i \times \mathbf{S}_j\right). \tag{7}$$

The Heisenberg coupling is given by

$$\begin{aligned} J_{ij}^H = -\frac{J^2}{4\pi} \int_{-\infty}^{\epsilon_F} d\omega \,\text{Im}\big\{ &\left[G_\uparrow^R\left(\mathbf{R}_i, \mathbf{R}_j, \omega\right) + G_\downarrow^R\left(\mathbf{R}_i, \mathbf{R}_j, \omega\right)\right] \left[G_\uparrow^R\left(\mathbf{R}_j, \mathbf{R}_i, \omega\right) + G_\downarrow^R\left(\mathbf{R}_j, \mathbf{R}_i, \omega\right)\right] \\ &- \left[G_\uparrow^R\left(\mathbf{R}_i, \mathbf{R}_j, \omega\right) - G_\downarrow^R\left(\mathbf{R}_i, \mathbf{R}_j, \omega\right)\right] \left[G_\uparrow^R\left(\mathbf{R}_j, \mathbf{R}_i, \omega\right) - G_\downarrow^R\left(\mathbf{R}_j, \mathbf{R}_i, \omega\right)\right]\big\}. \end{aligned} \tag{8}$$

The Ising-like coupling reads

$$J_{ij}^I = -\frac{J^2}{2\pi} \int_{-\infty}^{\epsilon_F} d\omega \,\text{Im}\left\{\left[G_\uparrow^R\left(\mathbf{R}_i, \mathbf{R}_j, \omega\right) - G_\downarrow^R\left(\mathbf{R}_i, \mathbf{R}_j, \omega\right)\right] \left[G_\uparrow^R\left(\mathbf{R}_j, \mathbf{R}_i, \omega\right) - G_\downarrow^R\left(\mathbf{R}_j, \mathbf{R}_i, \omega\right)\right]\right\}. \tag{9}$$

Finally, the Dzyaloshinskii-Moriya (DM) term is given by

$$\begin{aligned} J_{ij}^{DM} = -\frac{J^2}{4\pi} \int_{-\infty}^{\epsilon_F} d\omega \,\text{Im}\big\{ &i\left[G_\uparrow^R\left(\mathbf{R}_i, \mathbf{R}_j, \omega\right) + G_\downarrow^R\left(\mathbf{R}_i, \mathbf{R}_j, \omega\right)\right] \left[G_\uparrow^R\left(\mathbf{R}_j, \mathbf{R}_i, \omega\right) - G_\downarrow^R\left(\mathbf{R}_j, \mathbf{R}_i, \omega\right)\right] \\ &-i\left[G_\uparrow^R\left(\mathbf{R}_i, \mathbf{R}_j, \omega\right) - G_\downarrow^R\left(\mathbf{R}_i, \mathbf{R}_j, \omega\right)\right] \left[G_\uparrow^R\left(\mathbf{R}_j, \mathbf{R}_i, \omega\right) + G_\downarrow^R\left(\mathbf{R}_j, \mathbf{R}_i, \omega\right)\right]\big\}. \end{aligned} \tag{10}$$

Some features of the Hamiltonian in Eq. (7) must be pointed out at this point:

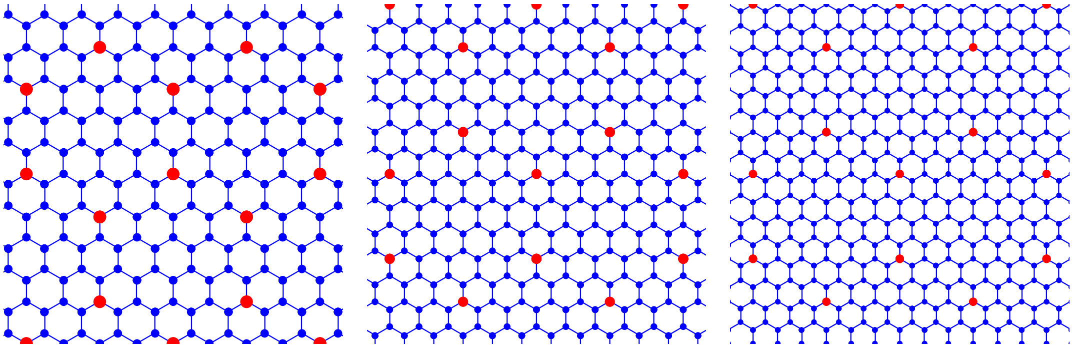

Figure 1: From left to right, super-lattice structures where the adatom-adatom distance is 4, 5 and 6 times the lattice spacing of silicene.

- This Hamiltonian is general. The only imposed constraint is the preservation of the $z \to -z$ mirror symmetry, which is incorporated in the model by means of the decomposition (6) of the Green operator.
- The second term in Eq. (6) is, to the leading order, proportional to the strength of the spin-orbit coupling (SOC) in the electronic system. Hence, according to Eq. (10), the DM term is first order in the SOC strength, whereas the anisotropy is second order, so that the latter can be safely neglected (at least in this realization of the model).
- A DM interaction with the full hexagonal ($D_{6h}$) symmetry requires the underlying electronic system to have a compatible symmetry. This is illustrated in the next 2 examples.

**Model 1: Adatoms on silicene**

Since we are trying to mimic a model originally proposed for graphene electrons, it is natural to consider as the simplest electronic system the $\mathbf{k} \cdot \mathbf{p}$ theory for itinerant electrons in a honeycomb lattice and in the presence of SOC,

$$\mathcal{H}_e = v_F \left( \pm \tau_x p_x + \tau_y p_y \right) \pm \Delta_{so} \tau_z \sigma_z, \tag{11}$$

where the sign $\pm$ applies to the two inequivalent valleys, and $\tau_{x,y,z}$ are Pauli matrices associated to the sublattice degree of freedom. In graphene, the SOC is very weak, $\Delta_{so} \sim \mu$eV; however, in silicene [1] it is of the order of meVs. This is due to the buckled structure of the lattice, which reduces the point group symmetry to $D_{3d}$. However, $D_{3d} \cong C_{6v}$; therefore, as long as we do not consider terms in the Hamiltonian that break expressly the mirror symmetry, the symmetries are compatible [2]. The hexagonal symmetry of the entire system –silicene and the lattice of adatoms– survives as long as both lattices share an inversion center. For simplicity, we consider super-lattice structures where the adatoms are placed on top of the silicon atoms as represented in Fig. 1. When the adatom-adatom distance $d$ is a multiple 3 of the silicon-silicon distance, the inversion centers do not coincide and then the symmetry of the super-structure is reduced from hexagonal to trigonal. Moreover, the calculation in that case gives $J_{ij}^{DM} = 0$ (note that all the adatoms are place on the same sublattice).

The Green functions in reciprocal space read

$$G_{sv\lambda}^{AA}(\mathbf{p},\omega) = \frac{\varepsilon(\mathbf{p}) + sv\lambda\Delta_{so}}{2\varepsilon(\mathbf{p})} \frac{1}{\omega + i0^+ - \lambda\varepsilon(\mathbf{p})},$$

$$G_{sv\lambda}^{BB}(\mathbf{p},\omega) = \frac{\varepsilon(\mathbf{p}) - sv\lambda\Delta_{so}}{2\varepsilon(\mathbf{p})} \frac{1}{\omega + i0^+ - \lambda\varepsilon(\mathbf{p})},$$

$$G_{sv\lambda}^{AB}(\mathbf{p},\omega) = \frac{\lambda v e^{-iv\phi(\mathbf{p})}}{2\varepsilon(\mathbf{p})} \frac{v_F|\mathbf{p}|}{\omega + i0^+ - \lambda\varepsilon(\mathbf{p})},$$

$$G_{sv\lambda}^{BA}(\mathbf{p},\omega) = \frac{\lambda v e^{iv\phi(\mathbf{p})}}{2\varepsilon(\mathbf{p})} \frac{v_F|\mathbf{p}|}{\omega + i0^+ - \lambda\varepsilon(\mathbf{p})},$$

where

$$\varepsilon(\mathbf{p}) = \sqrt{v_F^2 |\mathbf{p}|^2 + \Delta_{so}^2},$$
$$\phi(\mathbf{p}) = \arctan \frac{p_y}{p_x}.$$

Here $\mathbf{p}$ must be understood as the crystalline momentum around one of the valleys and $\lambda$, $v$, and $s$ label the band, valley and spin, respectively. By switching to the Fourier representation we obtain

$$G_{sv}^{AA}(\mathbf{R}_i, \mathbf{R}_j, \omega) = \sum_{\lambda=\pm 1} \int \frac{d^2\mathbf{p}}{(2\pi\hbar)^2} G_{sv\lambda}^{AA}(\mathbf{p}, \omega) e^{\frac{i\mathbf{p}\cdot(\mathbf{R}_i - \mathbf{R}_j)}{\hbar}} = -\frac{1}{2\pi} \frac{\omega + sv\Delta_{so}}{(\hbar v_F)^2} K_0 \left( \frac{|\mathbf{R}_i - \mathbf{R}_j|}{\hbar v_F} \sqrt{\Delta_{so}^2 - \omega^2} \right),$$
$$G_{sv}^{BB}(\mathbf{R}_i, \mathbf{R}_j, \omega) = \sum_{\lambda=\pm 1} \int \frac{d^2\mathbf{p}}{(2\pi\hbar)^2} G_{sv\lambda}^{BB}(\mathbf{p}, \omega) e^{\frac{i\mathbf{p}\cdot(\mathbf{R}_i - \mathbf{R}_j)}{\hbar}} = -\frac{1}{2\pi} \frac{\omega - sv\Delta_{so}}{(\hbar v_F)^2} K_0 \left( \frac{|\mathbf{R}_i - \mathbf{R}_j|}{\hbar v_F} \sqrt{\Delta_{so}^2 - \omega^2} \right),$$
$$G_{sv}^{AB}(\mathbf{R}_i, \mathbf{R}_j, \omega) = \sum_{\lambda=\pm 1} \int \frac{d^2\mathbf{p}}{(2\pi\hbar)^2} G_{sv\lambda}^{AB}(\mathbf{p}, \omega) e^{\frac{i\mathbf{p}\cdot(\mathbf{R}_i - \mathbf{R}_j)}{\hbar}} = \frac{ive^{-iv\theta_{ij}}}{2\pi(\hbar v_F)^2} \sqrt{\Delta_{so}^2 - \omega^2} K_1 \left( \frac{|\mathbf{R}_i - \mathbf{R}_j|}{\hbar v_F} \sqrt{\Delta_{so}^2 - \omega^2} \right),$$
$$G_{sv}^{BA}(\mathbf{R}_i, \mathbf{R}_j, \omega) = \sum_{\lambda=\pm 1} \int \frac{d^2\mathbf{p}}{(2\pi\hbar)^2} G_{sv\lambda}^{BA}(\mathbf{p}, \omega) e^{\frac{i\mathbf{p}\cdot(\mathbf{R}_i - \mathbf{R}_j)}{\hbar}} = \frac{ive^{iv\theta_{ij}}}{2\pi(\hbar v_F)^2} \sqrt{\Delta_{so}^2 - \omega^2} K_1 \left( \frac{|\mathbf{R}_i - \mathbf{R}_j|}{\hbar v_F} \sqrt{\Delta_{so}^2 - \omega^2} \right),$$

where $\theta_{ij}$ is the angle that $\mathbf{R}_j - \mathbf{R}_i$ makes with the $x$-axis (along the zig-zag direction in our geometry). It is worth mentioning at this point that the Green function in real space consists of the sum of the contributions coming from the two inequivalent valleys,

$$G_s^{\alpha\beta}(\mathbf{R}_i, \mathbf{R}_j, \omega) = e^{i\mathbf{K}\cdot(\mathbf{R}_i - \mathbf{R}_j)} G_{s,+1}^{\alpha\beta}(\mathbf{R}_i, \mathbf{R}_j, \omega) + e^{-i\mathbf{K}\cdot(\mathbf{R}_i - \mathbf{R}_j)} G_{s,-1}^{\alpha\beta}(\mathbf{R}_i, \mathbf{R}_j, \omega). \tag{12}$$

Next, we proceed to compute the Heisenberg and DM couplings to first and second nearest neighbors.

*Heisenberg coupling between 1st nearest neighbors*

From Eq. (8) we obtain, to the leading order in $\Delta_{so}$,

$$J_{ij}^H \approx -\frac{J^2}{4\pi} \int_{-\infty}^{\epsilon_F} d\omega \, \mathrm{Im} \left\{ \left[ G_\uparrow^{AB}(\mathbf{R}_i, \mathbf{R}_j, \omega) + G_\downarrow^{AB}(\mathbf{R}_i, \mathbf{R}_j, \omega) \right] \left[ G_\uparrow^{BA}(\mathbf{R}_j, \mathbf{R}_i, \omega) + G_\downarrow^{BA}(\mathbf{R}_j, \mathbf{R}_i, \omega) \right] \right\}. \tag{13}$$

For simplicity, we are assuming that the position $\mathbf{R}_i$ belongs to the $A$ sublattice and $\mathbf{R}_j$ to the $B$ sublattice. Then, we can write

$$J_{ij}^H(\mathbf{R} \equiv \mathbf{R}_B - \mathbf{R}_A) = \frac{[1 - \cos(2\mathbf{K}\cdot\mathbf{R} + 2\theta_{\mathbf{R}})] J^2}{2\pi^3 \hbar^4 v_F^4} \int_{-\infty}^{\epsilon_F} d\omega \, \mathrm{Im} \left\{ \left( \omega^2 - \Delta_{so}^2 \right) K_1^2 \left( \frac{R}{\hbar v_F} \sqrt{\Delta_{so}^2 - \omega^2} \right) \right\}. \tag{14}$$

For first nearest neighbors we have $1 - \cos(2\mathbf{K}\cdot\mathbf{R} + 2\theta_{\mathbf{R}}) = 2$. We consider the doped regime, characterized by $R \gg \frac{\hbar v_F}{\epsilon_F} \gg \frac{\hbar v_F}{\Delta_{so}}$. The asymptotic behavior of the coupling for long distances reads then

$$J_{ij}^H \approx -\frac{J^2}{2\pi\hbar v_F R^3} \int_0^{\frac{R\epsilon_F}{\hbar v_F}} dx x^2 J_1(x) Y_1(x) \approx -\frac{\epsilon_F J^2 \sin\left(\frac{2\epsilon_F R}{\hbar v_F}\right)}{4\pi^2 \hbar^2 v_F^2 R^2}. \tag{15}$$

*DM coupling between 2nd nearest neighbors*

In the case of the DM coupling between second nearest neighbors, we have to take into account which sublattice the adatoms are in, since there is a sign difference that can be immediately deduced from the expressions for the Green operators. We obtain

$$J_{ij}^{A-DM}(\mathbf{R} \equiv \mathbf{R}_j - \mathbf{R}_i) = -J_{ij}^{B-DM}(\mathbf{R} \equiv \mathbf{R}_j - \mathbf{R}_i) = \frac{\sin(2\mathbf{K}\cdot\mathbf{R}) \Delta_{so} J^2}{\pi^3 \hbar^4 v_F^4} \int_{-\infty}^{\epsilon_F} d\omega\omega \, \mathrm{Im} \left\{ K_0^2 \left( \frac{R}{\hbar v_F} \sqrt{\Delta_{so}^2 - \omega^2} \right) \right\}. \tag{16}$$

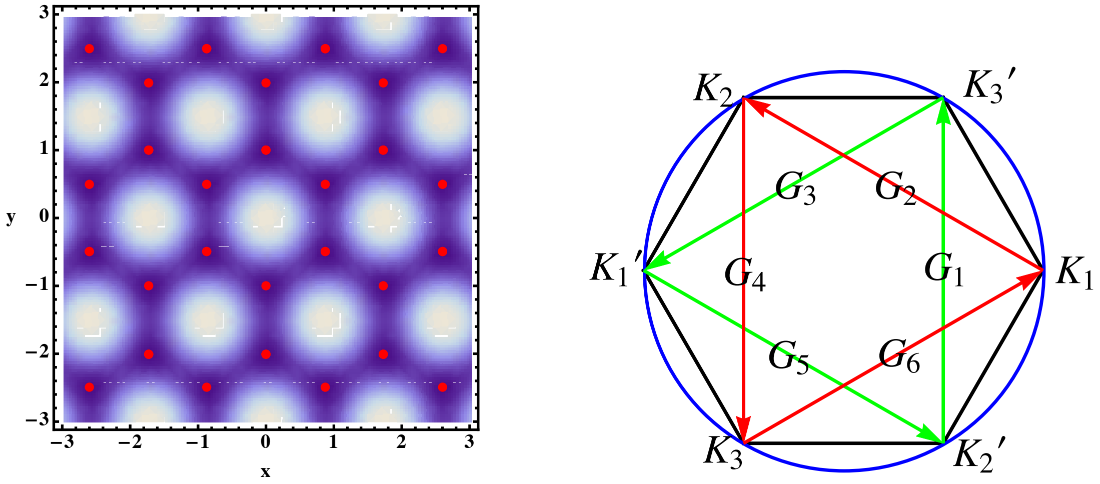


Figure 2: Left: Density plot of the potential in Eq. (19); the adatoms occupy the positions of minimum energy. Right: Sketch of the Brillouin zone of the superlattice.

For second nearest neighbors we have $\sin\left(2\mathbf{K}\cdot\left(\mathbf{R}_j-\mathbf{R}_i\right)\right)=\nu_{ij}\frac{\sqrt{3}}{2}$, where $\nu_{ij}$ is defined as in the main text. Finally, in the doped regime $R\gg\frac{\hbar v_F}{\epsilon_F}\gg\frac{\hbar v_F}{\Delta_{so}}$, we obtain

$$J_{ij}^{DM}\approx\frac{\sqrt{3}\Delta_{so}\nu_{ij}J^2}{2\pi\hbar^2v_F^2R^2}\int_0^{\frac{R\epsilon_F}{\hbar v_F}}dxxJ_0(x)Y_0(x)\approx-\frac{\sqrt{3}\Delta_{so}\nu_{ij}J^2\sin\left(\frac{2\epsilon_F R}{\hbar v_F}\right)}{4\pi^2\hbar^2v_F^2R^2}. \tag{17}$$

**Model 2: Heavy adatoms on a metal**

Another possibility is to consider a conventional parabolic dispersion for the surface states of a metal in the presence of a potential created by the adatoms. The Hamiltonian reads in general

$$\mathcal{H}=\frac{\mathbf{p}^2}{2m_*}+V\left(\mathbf{r}\right)+\frac{\hbar}{2m_*^2c^2}\mathbf{s}\cdot\left(\nabla V\left(\mathbf{r}\right)\times\mathbf{p}\right). \tag{18}$$

Here $V\left(\mathbf{r}\right)$ is a potential with the symmetry of the lattice of adatoms. Considering only the lowest harmonics, we can write

$$V\left(\mathbf{r}\right)=V\sum_{i=1}^{6}e^{i\mathbf{G}_i\cdot\mathbf{r}}. \tag{19}$$

This is an attractive potential created by the adatoms forming a honeycomb lattice, see Fig. 2. Here $\mathbf{G}_i$ are the first 6 reciprocal lattice vectors with lowest modulus. The last term in Eq. (18) is the SOC created by the heavy nuclei of the adatoms.

The original parabolic band is folded into the Brillouin zone of the super-lattice of adatoms. Hybridization gaps are open due to the action of the potential $V$, which can be understood within a nearly free electron picture. States with $\mathbf{p}/\hbar$ close to the edges of the new Brillouin zone are strongly modified since they lie in isoenergetic orbits. The process is depicted in the right panel of Fig. 2. The Hamiltonian for states close to $\mathbf{K}_{1,2,3}$ points, to linear order in $\mathbf{k}$ (crystalline momentum around these points), reads

$$\mathcal{H}_{\uparrow,\downarrow}^{\mathbf{K}}\left(\mathbf{k}\right)\approx\begin{pmatrix}\frac{\hbar^2|\mathbf{K}_1|^2}{2m_*}+\frac{\hbar^2\mathbf{K}_1\cdot\mathbf{k}}{m_*} & V\pm id^2V_{so}\mathbf{G}_5\times\mathbf{K}_2 & V\pm id^2V_{so}\mathbf{G}_6\times\mathbf{K}_3\\ V\pm id^2V_{so}\mathbf{G}_2\times\mathbf{K}_1 & \frac{\hbar^2|\mathbf{K}_2|^2}{2m_*}+\frac{\hbar^2\mathbf{K}_2\cdot\mathbf{k}}{m_*} & V\pm id^2V_{so}\mathbf{G}_1\times\mathbf{K}_3\\ V\pm id^2V_{so}\mathbf{G}_3\times\mathbf{K}_1 & V\pm id^2V_{so}\mathbf{G}_4\times\mathbf{K}_2 & \frac{\hbar^2|\mathbf{K}_3|^2}{2m_*}+\frac{\hbar^2\mathbf{K}_3\cdot\mathbf{k}}{m_*}\end{pmatrix}$$

$$=\begin{pmatrix}\frac{8\pi^2\hbar^2}{27d^2m_*}+\frac{4\pi\hbar^2}{3\sqrt{3}dm_*}k_x & V\pm i\frac{8\pi^2}{9\sqrt{3}}V_{so} & V\mp i\frac{8\pi^2}{9\sqrt{3}}V_{so}\\ V\mp i\frac{8\pi^2}{9\sqrt{3}}V_{so} & \frac{8\pi^2\hbar^2}{27d^2m_*}+\frac{4\pi\hbar^2}{3\sqrt{3}dm_*}\left(-\frac{k_x}{2}+\frac{\sqrt{3}}{2}k_y\right) & V\pm i\frac{8\pi^2}{9\sqrt{3}}V_{so}\\ V\pm i\frac{8\pi^2}{9\sqrt{3}}V_{so} & V\mp i\frac{8\pi^2}{9\sqrt{3}}V_{so} & \frac{8\pi^2\hbar^2}{27d^2m_*}+\frac{4\pi\hbar^2}{3\sqrt{3}dm_*}\left(-\frac{k_x}{2}-\frac{\sqrt{3}}{2}k_y\right)\end{pmatrix}, \tag{20}$$

where we have introduced $V_{so} \equiv \frac{\hbar^2 V}{2m_*^2 c^2 d^2}$. Similarly for $\mathbf{K}'_{1,2,3}$ points, we have

$$\mathcal{H}^{\mathbf{K}'}_{\uparrow,\downarrow}(\mathbf{k}) \approx \begin{pmatrix} \frac{\hbar^2\left|\mathbf{K}'_1\right|^2}{2m_*} + \frac{\hbar^2 \mathbf{K}'_1\cdot\mathbf{k}}{m_*} & V \pm id^2 V_{so}\mathbf{G}_2 \times \mathbf{K}'_2 & V \pm id^2 V_{so}\mathbf{G}_3 \times \mathbf{K}'_3 \\ V \pm id^2 V_{so}\mathbf{G}_5 \times \mathbf{K}'_1 & \frac{\hbar^2\left|\mathbf{K}'_2\right|^2}{2m_*} + \frac{\hbar^2 \mathbf{K}'_2\cdot\mathbf{k}}{m_*} & V \pm id^2 V_{so}\mathbf{G}_4 \times \mathbf{K}'_3 \\ V \pm id^2 V_{so}\mathbf{G}_6 \times \mathbf{K}'_1 & V \pm id^2 V_{so}\mathbf{G}_1 \times \mathbf{K}'_2 & \frac{\hbar^2\left|\mathbf{K}'_3\right|^2}{2m_*} + \frac{\hbar^2 \mathbf{K}'_3\cdot\mathbf{k}}{m_*} \end{pmatrix}$$

$$= \begin{pmatrix} \frac{8\pi^2\hbar^2}{27d^2m_*} - \frac{4\pi\hbar^2}{3\sqrt{3}dm_*}k_x & V \pm i\frac{8\pi^2}{9\sqrt{3}}V_{so} & V \mp i\frac{8\pi^2}{9\sqrt{3}}V_{so} \\ V \mp i\frac{8\pi^2}{9\sqrt{3}}V_{so} & \frac{8\pi^2\hbar^2}{27d^2m_*} + \frac{4\pi\hbar^2}{3\sqrt{3}dm_*}\left(\frac{k_x}{2} - \frac{\sqrt{3}}{2}k_y\right) & V \pm i\frac{8\pi^2}{9\sqrt{3}}V_{so} \\ V \pm i\frac{8\pi^2}{9\sqrt{3}}V_{so} & V \mp i\frac{8\pi^2}{9\sqrt{3}}V_{so} & \frac{8\pi^2\hbar^2}{27d^2m_*} + \frac{4\pi\hbar^2}{3\sqrt{3}dm_*}\left(\frac{k_x}{2} + \frac{\sqrt{3}}{2}k_y\right) \end{pmatrix}. \tag{21}$$

It is useful to diagonalize these Hamiltonians at $\mathbf{k} = 0$. For the $\mathbf{K}_{1,2,3}$ points we have:

$$\epsilon_a = \epsilon_0 \pm \frac{8\pi^2 V_{so}}{9} \qquad |a+\rangle = \frac{1}{\sqrt{3}}\left(|\mathbf{K}_1\rangle + e^{-2\pi i/3}|\mathbf{K}_2\rangle + e^{2\pi i/3}|\mathbf{K}_3\rangle\right)$$

$$\epsilon_b = \epsilon_0 \mp \frac{8\pi^2 V_{so}}{9} \qquad |b+\rangle = \frac{1}{\sqrt{3}}\left(|\mathbf{K}_1\rangle + e^{2\pi i/3}|\mathbf{K}_2\rangle + e^{-2\pi i/3}|\mathbf{K}_3\rangle\right)$$

$$\epsilon_c = \epsilon_0 + 3V \qquad |c+\rangle = \frac{1}{\sqrt{3}}\left(|\mathbf{K}_1\rangle + |\mathbf{K}_2\rangle + |\mathbf{K}_3\rangle\right), \tag{22}$$

where we have introduced $\epsilon_0 \equiv \frac{8\pi^2\hbar^2}{27d^2m_*} - V$. Analogously, for the $\mathbf{K}'_{1,2,3}$ points we obtain:

$$\epsilon_a = \epsilon_0 \mp \frac{8\pi^2 V_{so}}{9} \qquad |a-\rangle = \frac{1}{\sqrt{3}}\left(|\mathbf{K}'_1\rangle + e^{2\pi i/3}|\mathbf{K}'_2\rangle + e^{-2\pi i/3}|\mathbf{K}'_3\rangle\right)$$

$$\epsilon_b = \epsilon_0 \pm \frac{8\pi^2 V_{so}}{9} \qquad |b-\rangle = \frac{1}{\sqrt{3}}\left(|\mathbf{K}'_1\rangle + e^{-2\pi i/3}|\mathbf{K}'_2\rangle + e^{2\pi i/3}|\mathbf{K}'_3\rangle\right)$$

$$\epsilon_c = \epsilon_0 + 3V \qquad |c-\rangle = \frac{1}{\sqrt{3}}\left(|\mathbf{K}'_1\rangle + |\mathbf{K}'_2\rangle + |\mathbf{K}'_3\rangle\right) \tag{23}$$

In the absence of SOC effects ($V_{so} = 0$), states $a$ and $b$ form a doublet protected by the $C_{6v}$ symmetry. The $\mathbf{k} \cdot \mathbf{p}$ theory corresponds to a Dirac Hamiltonian and the SOC coupling opens a Kane-Mele gap. The effective Hamiltonian describing these states is given by Eq. (11) with parameters

$$v_F = \frac{2\pi\hbar}{3dm_*}, \tag{24}$$

$$\Delta_{so} = \frac{8\pi^2 V_{so}}{9}. \tag{25}$$

If we consider now that the Fermi level of the system lies close to $\epsilon_0$, then we can use this simplified Hamiltonian in order to compute the couplings. The calculation is very similar to the one performed in the previous section. Notice, however, that now the analogue of the *sublattice* degree of freedom does not correspond to a real sublattice; it is an internal quantum number with respect to which we have to perform a trace in the calculation.

*Heisenberg coupling between 1st nearest neighbors*

For the exchange coupling, we have

$$J^H_{ij} \approx -\frac{J^2}{4\pi}\sum_{\alpha,\beta=a,b}\int_{-\infty}^{\epsilon_F} d\omega \ \mathrm{Im}\left\{\left[G^{\alpha\beta}_{\uparrow}(\mathbf{R}_i,\mathbf{R}_j,\omega) + G^{\alpha\beta}_{\downarrow}(\mathbf{R}_i,\mathbf{R}_j,\omega)\right]\left[G^{\beta\alpha}_{\uparrow}(\mathbf{R}_j,\mathbf{R}_i,\omega) + G^{\beta\alpha}_{\downarrow}(\mathbf{R}_j,\mathbf{R}_i,\omega)\right]\right\}. \tag{26}$$

This last equation can be recast as

$$J^H_{ij} = -\frac{J^2}{4\pi^3\hbar^4 v_F^4}\left[\left(|f_a(\mathbf{R}_i,\mathbf{R}_j)|^2 + |f_b(\mathbf{R}_i,\mathbf{R}_j)|^2\right) \times \int_{-\infty}^{\epsilon_F} d\omega\omega^2 \ \mathrm{Im}\ K_0^2\left(\frac{R}{\hbar v_F}\sqrt{\Delta_{so}^2 - \omega^2}\right)\right.$$
$$\left. - \left(|f_{ab}(\mathbf{R}_i,\mathbf{R}_j)|^2 + |f_{ab}(\mathbf{R}_j,\mathbf{R}_i)|^2\right) \times \int_{-\infty}^{\epsilon_F} d\omega\omega^2 \ \mathrm{Im}\ K_1^2\left(\frac{R}{\hbar v_F}\sqrt{\Delta_{so}^2 - \omega^2}\right)\right], \tag{27}$$

where we have introduced the following functions:

$$f_a(\mathbf{R}_i,\mathbf{R}_j) = \sum_{v=\pm1} \langle \mathbf{R}_i | av\rangle\langle av | \mathbf{R}_j\rangle , \tag{28}$$

$$f_b(\mathbf{R}_i,\mathbf{R}_j) = \sum_{v=\pm1} \langle \mathbf{R}_i | bv\rangle\langle bv | \mathbf{R}_j\rangle , \tag{29}$$

$$f_{ab}(\mathbf{R}_i,\mathbf{R}_j) = \sum_{v=\pm1} ive^{-iv\theta_{ij}} \langle \mathbf{R}_i | av\rangle\langle bv | \mathbf{R}_j\rangle . \tag{30}$$

For first nearest neighbors we have $f_a(\mathbf{R}_i,\mathbf{R}_j) = f_b(\mathbf{R}_i,\mathbf{R}_j) = 0$ and $|f_{ab}(\mathbf{R}_i,\mathbf{R}_j)|^2 + |f_{ab}(\mathbf{R}_j,\mathbf{R}_i)|^2 = 36$. Therefore, the coupling reduces to

$$J_{ij}^{H} = \frac{9J^2}{\pi^3\hbar^4 v_F^4}\int_{-\infty}^{\epsilon_F} d\omega\omega^2 \,\mathrm{Im}\, K_1^2\left(\frac{d}{\hbar v_F}\sqrt{\Delta_{so}^2-\omega^2}\right), \tag{31}$$

which, in the doped regime $R \gg \frac{\hbar v_F}{\epsilon_F} \gg \frac{\hbar v_F}{\Delta_{so}}$, becomes

$$J_{ij}^{H} \approx -\frac{9\epsilon_F J^2 \sin\left(\frac{2\epsilon_F d}{\hbar v_F}\right)}{4\pi^2\hbar^2 v_F^2 d^2} = -\left(\frac{3}{2\pi}\right)^4 \frac{\epsilon_F J^2 m_*^2}{\hbar^4}\sin\left(\frac{3d^2 m_*\epsilon_F}{\pi\hbar^2}\right). \tag{32}$$

The final result is written in terms of parameters of the original model, Eq. (18). The Fermi level $\epsilon_F$ is measured with respect to the Dirac point.

*DM coupling between 2nd nearest neighbors*

For the DM coupling to the leading order in $\Delta_{so}$, we have

$$\begin{aligned} J_{ij}^{DM} \approx -\frac{J^2}{4\pi}\sum_{\alpha=a,b}\int_{-\infty}^{\epsilon_F} d\omega \,\mathrm{Im}\left\{ i\left[G_\uparrow^{\alpha\alpha}(\mathbf{R}_i,\mathbf{R}_j,\omega) + G_\downarrow^{\alpha\alpha}(\mathbf{R}_i,\mathbf{R}_j,\omega)\right]\left[G_\uparrow^{\alpha\alpha}(\mathbf{R}_j,\mathbf{R}_i,\omega) - G_\downarrow^{\alpha\alpha}(\mathbf{R}_j,\mathbf{R}_i,\omega)\right]\right. \\ \left. -i\left[G_\uparrow^{\alpha\alpha}(\mathbf{R}_i,\mathbf{R}_j,\omega) - G_\downarrow^{\alpha\alpha}(\mathbf{R}_i,\mathbf{R}_j,\omega)\right]\left[G_\uparrow^{\alpha\alpha}(\mathbf{R}_j,\mathbf{R}_i,\omega) + G_\downarrow^{\alpha\alpha}(\mathbf{R}_j,\mathbf{R}_i,\omega)\right]\right\}, \end{aligned} \tag{33}$$

which can be recast as

$$J_{ij}^{DM} = \frac{\Delta_{so}J^2\left[\sum_\alpha \mathrm{Im}\, f_{\alpha\alpha}(\mathbf{R}_i,\mathbf{R}_j)\right]}{2\pi^3\hbar^4 v_F^4}\int_{-\infty}^{\epsilon_F} d\omega\omega \,\mathrm{Im}\left\{K_0^2\left(\frac{R}{\hbar v_F}\sqrt{\Delta_{so}^2-\omega^2}\right)\right\}. \tag{34}$$

The function $f_{\alpha\alpha}$ is defined as:

$$f_{\alpha\alpha}(\mathbf{R}_i,\mathbf{R}_j) = \begin{cases} \left(\sum_{v=\pm1}\langle \mathbf{R}_i | \alpha v\rangle\langle \alpha v | \mathbf{R}_j\rangle\right)\left(\sum_{v=\pm1} v\,\langle \mathbf{R}_i | \alpha v\rangle\langle \alpha v | \mathbf{R}_j\rangle\right) & \text{if } \alpha = a \\ -\left(\sum_{v=\pm1}\langle \mathbf{R}_i | \alpha v\rangle\langle \alpha v | \mathbf{R}_j\rangle\right)\left(\sum_{v=\pm1} v\,\langle \mathbf{R}_i | \alpha v\rangle\langle \alpha v | \mathbf{R}_j\rangle\right) & \text{if } \alpha = b \end{cases} \tag{35}$$

For first nearest neighbors we have $\sum_\alpha \mathrm{Im}\, f_{\alpha\alpha}(\mathbf{R}_i,\mathbf{R}_j) = 0$, whereas for second nearest neighbors $\sum_\alpha \mathrm{Im}\, f_{\alpha\alpha}(\mathbf{R}_i,\mathbf{R}_j) = 9\sqrt{3}\nu_{ij}$. Therefore, in the doped regime, $R \gg \frac{\hbar v_F}{\epsilon_F} \gg \frac{\hbar v_F}{\Delta_{so}}$, we obtain

$$J_{ij}^{DM} \approx -\frac{3\sqrt{3}\Delta_{so}\nu_{ij}J^2\sin\left(\frac{2\sqrt{3}\epsilon_F d}{\hbar v_F}\right)}{4\pi^2\hbar^2 v_F^2 d^2} = -\frac{3\sqrt{3}}{2\pi^2}\nu_{ij}\frac{V_{so}J^2 m_*^2}{\hbar^4}\sin\left(\frac{3\sqrt{3}\epsilon_F d^2 m_*}{\pi\hbar^2}\right). \tag{36}$$

---

[1] Motohiko Ezawa, Phys. Rev. Lett. **109**, 055502 (2012).
[2] Note that there is also a Rashba-like SOC of the form $\sigma_z(k_x s_y - k_y s_x)$ allowed by $D_{3d}$ symmetry that breaks explicitly the symmetry $z \to -z$. However, its strength is at least an order of magnitude less than the Kane-Mele coupling (both can be seen as spin/sublattice-dependent hoppings between second nearest neighbors), and it is absent at the band edges, so it can be safely neglected for moderate dopings.
